# Supplementary material for: Covariate Distribution Aware Meta-learning
Source: arXiv:2007.02523 source file (2020-11-28)
Supplement: Supplementary file 1 [file appendix.tex]

\section{Appendix}
\subsection{Regression Benchmark}
Here we provide a detailed description of the regression dataset discussed in Sec.~\ref{sec:experiments}. It has been adapted from \cite{vuorio2019multimodal}. As mentioned in Sec.~\ref{sec:experiments}, for each task we first sample the covariates ($x \in \C{R}$) from $\C{N}(\mu_\C{T}, \sigma_{\C{T}})$. Then, the optimal hypothesis for each task is sampled from one of the modalities or hypothesis classes. The hypothesis classes considered are : \textit{sine}, \textit{linear}, \textit{quad}, \textit{transformed-L$_1$} and \textit{tanh}. For each task, having chosen a hypothesis class, the parameters of the optimal hypothesis (like slope of a linear function) are chosen based on uniform distributions over the following:
% \setlist{nolistsep}
\begin{enumerate}
    \item \textit{sine}: $f(x)=A\cdot(sin (w \cdot x) + b)$, with $A \in [0.1, 5.0], w \in [0.5, 2.0]$ and $b \in [0, 2\pi]$.
    \item \textit{quad}: $f(x)=A\cdot(x - c)^2 + b$ with 
 $A \in [-0.15, -0.02] \cup [0.02, 0.15], c \in [-3.0, 3.0]$ and $b \in [-3.0, 3.0]$.
    \item \textit{linear}: $f(x) = A \cdot x + b$, $A \in [-3, 3], b \in [-3, 3]$.
    \item \textit{transformed-L$_1$}: $f(x)=A \cdot |x - c| + b$, with $A \in [-0.15, -0.02] \cup [0.02, 0.15], c \in [-3.0, 3.0]$ and $b \in [-3.0, 3.0]$.
    \item \textit{tanh}: $f(x) = A \cdot tanh(x-c)+b$ with $A \in [-3.0, 3.0], c \in [-3.0, 3.0], b \in [-3.0, 3.0]$.
\end{enumerate}
For each of the true hypothesis classes above the final value of $\V{y}^{(i)}_j$ is generated by adding an independent error term $\epsilon$ sampled from a normal distribution with mean $0$ and standard deviation of $0.3$ \textit{i.e} $\V{y}_j^{(i)} = f(\V{x}_j^{(i)}) + \epsilon$. From the above formulation we can clearly see that the optimal hypothesis for a task is dependent on the corresponding covariate distribution for it. Thus, the ideal initialization that can converge to the optimal task parameters in a few steps of gradient descent is also dependent on the covariate distribution.

Based on the description of the tasks above, we form two sets of three different datasets (each) and study them separately as two different cases described in Sec.~\ref{sec:experiments}. Each of the three datasets have different complexities depending on the number of modalities (hypothesis classes) that the optimal hypothesis for a task can be sampled from. These are described as follows:
\begin{enumerate}
    \item \textit{sine}: true hypothesis for each task is given by a sinusoidal function with parameters sampled from distributions mentioned previously. However, the domain for each of the parameters is split into $P=3$ disjoint sets. 
    \item \textit{sine-quad-linear}: true hypothesis for each task is restricted to only three classes: \textit{sine, quad} and \textit{linear}.
    \item \textit{five}: all five hypothesis classes are considered
\end{enumerate}

To highlight the benefits of our meta-learning algorithm, let's consider \textbf{Case-I} (Sec.~\ref{sec:experiments}) where a relation exists between the covariate distribution and the hypothesis class. Each hypothesis class is mapped to a class of covariate distributions. For example, for a given task if the true hypothesis lies in the \textit{quad} class, then the covariates for that task can be sampled from $x \sim \C{N}(-7,1)$. On the other hand, if the true hypothesis is given by a \textit{linear} function, then the covariates are sampled from a different region $x \sim \C{N}(7,3)$. Apart from this case, where we we can clearly see the gains of our proposed approach, we also study the case (\textbf{Case-II}) where no explicit relation exists between the optimal hypothesis classes and the covariate distributions of tasks. 

% For The datasets are listed as follows:
% \setlist{nolistsep}
% \begin{enumerate}
%     \item \textit{sine}: true hypothesis for each class is given by a sinusoidal function with parameters sampled from distributions mentioned previously. The range for each of the parameters is split into $P=3$ disjoint sets, each one corresponding to a specific covariate distribution. 
%     \item \textit{sine-quad-linear}: each of the three hypothesis classes are mapped to a specific covariate distribution. Thus, once the parameters of the covariate distribution are sampled based on the discrete prior, the corresponding hypothesis class is also chosen and a task is sampled from it.
%     \item \textit{five}: similar to the previous case with the distinction that all five hypothesis classes are considered in this dataset \textit{i.e} $P=5$.
% \end{enumerate}


\subsection{Additional Hyper-parameter Details}

All models were trained using SGD with momentum $(=0.9)$ for a total of 60 epochs with 1000 iterations per epoch. The initial learning rate was set to 0.1 which was further reduced to 0.006 at epoch 20 and 0.0012 at epoch 40. The reported numbers are the test evaluations for the best performing models on the validation splits. Both validation and test performances were evaluated using a total of 1000 tasks with 500 query points and 1 (for \textbf{5w1s}) or 5 (for \textbf{5w5s}) support points per task. Data augmentation was not applied to any of the runs but based on other works we believe that augmenting the dataset with random crops and horizontal flips can further reduce the generalization gap (especially for the deeper backbones). For all methods, the inner optimization loop involved 5 updates and an $l_2$ penalty or weight decay of $0.5 \times 10^{-3}$ was also added on the entire set of meta-parameters.




\subsection{Results on a Deeper Network}

In order to evaluate our approach for deeper feature extractors we experiment with the Resnet-12 architecture. Most initialization based methods \cite{finn2017model, finn2018probabilistic, vuorio2019multimodal, ravi2018amortized} were originally proposed for shallower architectures like Conv64 which has 4 convolution layers. Since Resnet-12 suffers from an extremely high dimensional parameter space, optimizing a meta-learning method to learn an optimal initialization in this space can be a potentially ill-conditioned problem. This is probably the reason why the benefits of using a deeper backbone is less clear when compared to some of the meta-learning methods that learn only the last-layer parameters for each task \cite{lee2019meta,snell2017prototypical}. Notwithstanding, even with a deeper architecture we demonstrate the superior performance of our approach as compared to other initialization based methods on the \textbf{miniImageNet} dataset (Table \ref{tab:classification-results-resnet-mi}).



\begin{table}[!ht]
    \centering
    {\setlength{\tabcolsep}{0.4em}
    \begin{tabular}{ c  c  c}
    \textbf{Model}     & \textbf{5w5s}  & \textbf{5w1s} \\\toprule
    \textsc{maml}    &  $67.50 \pm 0.35 \%$ &   $51.99 \pm 0.41 \%$     \\
    \textsc{reptile}    &  $67.31 \pm 0.44 \%$ &   $52.05 \pm 0.35 \%$     \\
    \textsc{m-maml}   &   $66.29 \pm 0.34 \%$ &   $51.86 \pm 0.38 \%$ \\ \midrule
    Ours &  $\V{68.12 \pm 0.43 \%}$ &   $\V{52.48 \pm 0.50 \%}$   
    \end{tabular}}
    \caption{Comparison (based on the Resnet-12 backbone) to prior work on \textbf{miniImagenet} dataset denoting the mean few-shot classification accuracies (in $\%$) along with their $95\%$ confidence intervals on \textbf{5w5s} and \textbf{5w1s} tasks. All reported values for the baselines are based on our re-implementation.}
  \label{tab:classification-results-resnet-mi}
\end{table}



% \begin{table}[!ht]
%     \centering
%     {\setlength{\tabcolsep}{0.4em}
%     \begin{tabular}{ c  c  c}
%     \textbf{Model}     & \textbf{5w5s}  & \textbf{5w1s} \\\toprule
%     \textsc{maml}   &   $77.41 \pm 0.32 \%$ &   $57.60 \pm 0.57 \%$   \\
%     \textsc{m-maml}  &    $79.38 \pm 0.35 \%$ &   $58.15 \pm 0.39 \%$ \\ \midrule
%     Ours &  $79.91 \pm 0.30 \%$ &   $57.01 \pm 0.38 \%$   
%     \end{tabular}}
%     \caption{Comparison (based on the Resnet-12 backbone) to prior work on \textbf{CUB} dataset denoting the mean few-shot classification accuracies (in $\%$) along with their $95\%$ confidence intervals on \textbf{5w5s} and \textbf{5w1s} tasks.}
%   \label{tab:classification-results-resnet-cub}
% \end{table}


% \subsection{}
